# Supplementary material for: Generalized Precision Matrix for Scalable Estimation of Nonparametric Markov Networks
Source: arXiv:2305.11379 source file (2023-05-19)
Supplement: Supplementary file 1 [file draft_appendix.tex]

\section{Notes \textcolor{red}{(To be removed)}}
\subsection{Connection between Markov Network and Causal DAG}
Let $(\mathcal{M}, \mathbb{P}_\mathbf{X})$ be the Markov network over $d$ variables, denoted as $\mathbf{X}=\{X_1,\dots,X_d\}$, where $\mathcal{M}$ is an undirected graph. Assume that this Markov network corresponds to a Bayesian network $(\mathcal{B}, \mathbb{P}_\mathbf{X})$, where $\mathcal{B}$ is a DAG. Under certain assumptions to be determined (possibly include the single shielded-collider-faithfulness and single unshielded-collider-faithfulness assumptions), $\mathcal{M}$ is the moralized graph of DAG $\mathcal{B}$. 

The goal is to develop an effecient procedure to discover the DAG $\mathcal{B}$ from the undirected graph $\mathcal{M}$, under assumption such as faithfulness. In other words, the goal is to discover the v-structures (of DAG $\mathcal{B}$) in undirected graph $\mathcal{M}$. In this case, it suffices to consider the triangles in $\mathcal{M}$. 

Suppose $X_1\rightarrow X_2\leftarrow X_3$ forms a v-structure (unshielded collider) in DAG $\mathcal{B}$, which correspond to a triangle in undirected graph $\mathcal{M}$. The goal is to determine the non-adjacent pairs ($X_1$ and $X_3$) in this triangle.

Case 1: Consider the adjacent pair, say $X_1$ and $X_2$ in the triangle. Clearly, no conditioning set $\mathbf{S}\subseteq \mathbf{X}\setminus\{X_1,X_2,X_3\}$ can separate these two variables in $\mathcal{M}$. That is, for all $\mathbf{S}\subseteq \mathbf{X}\setminus\{X_1,X_2,X_3\}$, we have $X_1\notindependent X_2|\mathbf{S}$, under the adjacency faithfulness assumption.

Case 2: Consider the non-adjacent pair, say $X_1$ and $X_3$ in the triangle. Since they are non-adjacent, there must be a conditioning set that separates them in undirected graph $\mathcal{M}$, or d-seprates them in DAG $\mathcal{B}$. \emph{The goal is then to find this conditioning set efficiently from the Markov network}, which we denote by $\mathbf{S}\subseteq \mathbf{X}\setminus\{X_1,X_2,X_3\}$. Excluding $X_2$, suppose that there are $k$ other undirected paths between $X_1$ and $X_3$ in $\mathcal{M}$, denoted as $P_1,\dots,P_k$, where $P_i=(P_{i,1},\dots,P_{i,\ell_i})$ for $i=[k]$. Here, $\ell_i$ indicates the length of path $P_i$, and $P_{i,j}$ refers to any variable from $\mathbf{X}\setminus \{X_1,X_2,X_3\}$.
\begin{itemize}
\item For any path $P_i$, if both $X_1, X_3, P_{i,1}$ and $X_1, X_3, P_{i,\ell_i}$ do not form a triangle in undirected graph $\mathcal{M}$, then conditioning on all variables $\{P_{i,1},\dots,P_{i,\ell_i}\}$ will block the path $P_i$. Therefore, we could simply include these variables in the set $\mathbf{S}_1$, which will be later included in the final conditioning set.
\item For any path $P_i$, if it contains only one variable, then we add $P_{i,1}$ to a separate set $\mathbf{S}_2$ (which we will later choose from).
\item For any path $P_i$, if either $X_1, X_3, P_{i,1}$ or $X_1, X_3, P_{i,\ell_i}$ forms a triangle in undirected graph $\mathcal{M}$, then we add $P_{i,1}$ and $P_{i,\ell_i}$ to a separate set $\mathbf{S}_2$ (which we will later choose from).
\end{itemize}
Now we have two sets $\mathbf{S}_1$ and $\mathbf{S}_2$, and we would like to create a final conditioning set $\mathbf{S}$. We sample any number of variables from $\mathbf{S}_2$, and denote the resulting set as $\mathbf{S}_2'\subseteq \mathbf{S}_2$. We then create the set $\mathbf{S}=\mathbf{S}_1\cup \mathbf{S}_2'$, and test whether $X_1\independent X_3|\mathbf{S}$. This indicates that we have to perform $2^{|\mathbf{S}_2|}$ conditional independence tests at most. If, for any set $\mathbf{S}$, we have $X_1\independent X_3|\mathbf{S}$, then we can conclude that $X_1\rightarrow X_2\leftarrow X_3$ is a v-structure (unshielded collider) in DAG $\mathbf{B}$ (under faithfulness assumption). Otherwise, $X_1$ and $X_3$ are adjacent in DAG $\mathbf{B}$.

\textcolor{red}{Note: The first and third bullet points may be further optimized. For the third bullet point, adding both $P_{i,1}$ and $P_{i,\ell_i}$ might be redundant in some cases.}

\textcolor{red}{Note: By doing this, we would like to minimize the number of independence tests we need given a sound markov network. To put it under the same umbrella of score matching and the proposed statistics, we need to first deal with conditioning sets that are subsets of the remaining variables.}
